# Supplementary material for: Heating of Cs2Te Photocathode via Field Emission and RF Pulsed Heating: Implication Toward Breakdown
Source: arXiv:2503.02761 source file (2025-03-04)
Supplement: Supplementary file 1 [file appendix.tex]

\appendix
\counterwithin{figure}{section}

\section{Analytical Pulsed Heating Calculation} \label{appendix:pulsed_heating}
For a standing wave cavity, the rise and fall of the magnetic field amplitude during a pulse can be written as \cite{analyticalRFpulsedheating}
\begin{equation}
H_0(t)=
    \begin{cases}
        H_0(1-e^{-\frac{t}{\tau}}), &  t < t_{p}\\
        H_0(1-e^{-\frac{t_{p}}{\tau}})e^{-\frac{t-t_{p}}{\tau}}, & t > t_{p}
    \end{cases}
\end{equation}
where $\tau$ is the filling time of a RF cavity and $t_{p}$ is the pulse length. The heat diffusion equation Eq. \ref{eq:heat_diffusion} can be solved for a metallic slab with finite width $L$, giving us the temperature increase and decrease on the substrate. Here, the heat source $f(x,t)$ is given by the the average power dissipated per unit area due to the electro-magnetic field,
\begin{align}
    f(x,t)=\frac{P(x,t)}{\rho C_V}\notag \\
    P(x,t)=\frac{R_s}{\delta}H_0(t)^2e^{-2x/\delta}
\end{align}
where, $R_s$ is the surface resistance and $\delta$ is the skin depth. The solution to such problem have been solved in \cite{analyticalRFpulsedheating} giving us the transient temperature,

\begin{align} \label{eq:PH_single}
    \Delta T(x,t) &= a_0(t) +\sum_{n=1}^{\infty} a_n(t)cos \left( \frac{\pi nx}{L} \right), \: t < t_{p}\notag \\
    \Delta T(x,t) &= a_0(t_p)+\frac{1}{2}b_0(t-t_p)\notag \\
    &+ \sum_{n=1}^{\infty}\left(b_n(t-tp)+a_n(t_p)e^{-M_n^2(t-t_p)}\right)\notag \\
    &\times cos \left( \frac{\pi nx}{L} \right), \: t > t_{p}
\end{align}

where,
%\begin{equation}
\begin{align}
    D &= \sqrt{\frac{\kappa}{\rho C_e}}, \: M_n = \frac{\pi n}{L} D\notag \\
    c_0&= \frac{R_s|H_0|^2}{\rho C_e L}(1-e^{-\frac{2L}{\delta}})\notag \\
    c_n&= \frac{4 R_s L}{\rho C_e (4L^2 +(\pi \delta n)^2)}(1-e^{-\frac{2L}{\delta} (-1^n)})\notag \\
    a_0(t)&= \frac{c_0}{2} \left[t+\tau \left(2e^{-t/\tau}-\frac{1}{2}e^{-2t/\tau}-\frac{3}{2}\right)\right]\notag \\
    a_n(t)&=\frac{c_n}{M_n^2}\left(1-e^{-M_n^2 t} \right) + \frac{c_n}{M_n^2} \left(e^{-2t/\tau} -e^{-M_n^2 t} \right)\notag\\
          &+ \frac{2 c_n}{M_n^2 -1/\tau}\left(e^{-M_n^2t-e^{-t/\tau}}\right)\notag\\
    b_n(t)&=\frac{c_n(1-e^{-tp/t})^2}{M_n^2-2/\tau} \left(e^{-2t/\tau}-e^{M_n^2t}\right)
\end{align}
%\end{equation}
Fig. \ref{fig_pulsed_heating}(a) reports an example of temperature rise on the metal substrate surface when $H_0=400$ kA/m, $L=1$ cm, $C_e=380$ J/kg/K, $\delta=0.595$ $\mu$m, $\kappa = 400$ W/m/K, and $t_p=400$ ns.

\begin{figure}
	\includegraphics[width=8.6cm]{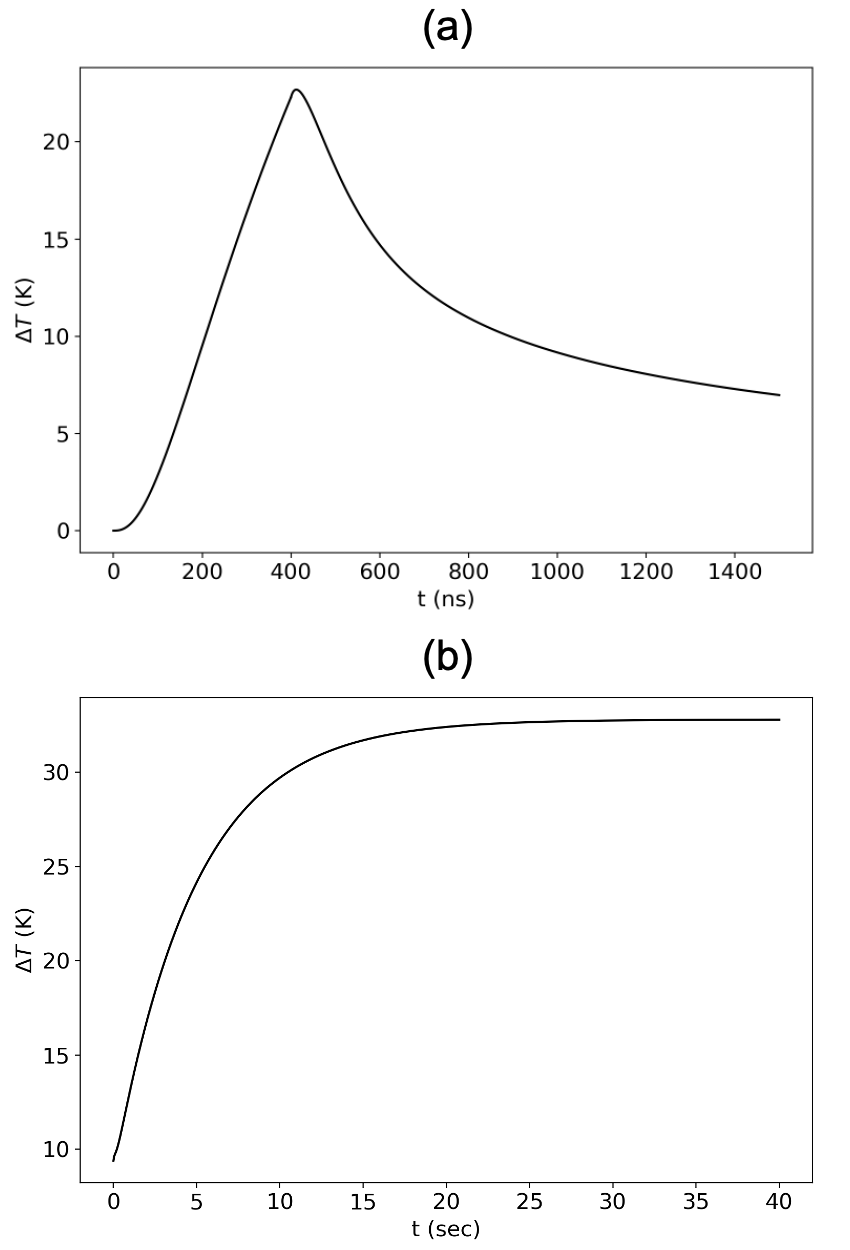}
	\caption{Energy  diagrams of semiconductor emitter in a strong electric field for p-type semiconductors}
	\label{fig_pulsed_heating}
\end{figure}

Similarly, the temperature increase when the accelerating structure is operated for many RF pulses over operational period $t_{\text{end}}$ can be obtain by solving the heat diffusion equation under an assumption that time varying heat source can be approximated by the time-average of the generated heat during the total operational time, 
\begin{align}
    q_{0}&=\frac{1}{t_{\text{end}}} \int_0^{t_{\text{end}}} \int_0^L P(x,t) dt dx \notag \\
         &=\frac{1}{t_{\text{end}}} \int_0^{t_{\text{end}}} H_0(t) dt \int_0^L \frac{R_s}{\delta}e^{-2x/\delta} dx 
\end{align}
Again, this problem have been solved in \cite{analyticalRFpulsedheating} with the solution to the partial differential equation given as,
\begin{subequations}
\begin{align}
    \Delta T(x,t) &= \frac{q_0}{\kappa}\left( L +\frac{\kappa}{h}\right)-\frac{q_0}{\kappa}x\notag \\
    &+ \sum_{n=1}^\infty C_n cos(k_n x)e^{-(Dk_n)^2 t} \\
    C_n &= \frac{ \left(
    \splitfrac{\frac{1}{k_n}sin(k_n L)(T_0-T'_\infty)}
    {- \frac{q_0}{k_n^2 \kappa} (1-\left(1+\frac{hL}{\kappa}\right)cos(k_n L))} \right)} {(\frac{L}{2} + \frac{sin(2k_n L)}{4k_n})}  \\
    & k_n tan(k_n L) = \frac{h}{\kappa} \label{eq:transcendental} \\
    & T'_\infty = \frac{q_0}{\kappa}\left( L +\frac{\kappa}{h}\right)
\end{align}
\end{subequations}
Here, the solutions to the transcendental Eq. \ref{eq:transcendental} are solved numerically utilizing Mathematica function \textit{FindInstant}. An example of temperature increase and subsequent saturation as $t\rightarrow \infty$ is shown in Fig. \ref{fig_pulsed_heating}(b) where pulse frequency of $f_p=400$ Hz is used to approximate the time-averaged heat generation. Rest of the parameters remains the same the single pulse example reported in Fig. \ref{fig_pulsed_heating}(a).

\addcontentsline{toc}{section}{Appendices}
